# Supplementary material for: Needmining: Designing Digital Support to Elicit Needs from Social Media
Source: arXiv:2101.06146 source file (2021-01-14)
Supplement: Supplementary file 1 [file appendix.tex]

\section*{Appendix}

\begin{table}[htbp]
	\caption{Overview of preprocessing options and their implementation}
	\centering
	\includegraphics[width=0.5\textwidth]{gfx/preprocessing_implementations}
	\label{fig:preprocessing_implementations}
\end{table}

\begin{table}[htbp]
	\centering
	\caption{Quantitative share of the major need categories and the needs, n=1,093}
	\label{tab:tweetresultsml}
	\begin{adjustbox}{width=1\textwidth}
		\begin{tabular}{|l|l|l|r|}
			\hline
			\textbf {Major Need Category} & \textbf {Amount (Share)} & \textbf {Need} & \textbf {Amount (Share)} \\
			\hline
			\multirow{4}{*}{price}                   & \multirow{4}{*}{202 (14.8\%)} & car price                                       & 154 (11.2\%) \\ \cline{3-4} 
			& \multicolumn{1}{c|}{}                        & electrical price                                & 22 (1.6\%)  \\ \cline{3-4} 
			& \multicolumn{1}{c|}{}                        & price (other)                                   & 22 (1.6\%)  \\ \cline{3-4} 
			& \multicolumn{1}{c|}{}                        & oil/gas price                                   & 4 (0.3\%)  \\ \hline
			\multirow{7}{*}{car characteristics}     & \multirow{7}{*}{145 (10.6\%)}                      & car characteristics (other)                     & 66 (4.8\%)  \\ \cline{3-4} 
			&                                              & car design                                      & 28 (2.0\%)  \\ \cline{3-4} 
			&                                              & car sound                                       & 19 (1.4\%)  \\ \cline{3-4} 
			&                                              & driving experience                              & 15 (1.1\%)  \\ \cline{3-4} 
			&                                              & car comfort                                     & 7 (0.5\%)  \\ \cline{3-4} 
			&                                              & car performance                                 & 6 (0.4\%)  \\ \cline{3-4} 
			&                                              & car smell                                       & 4 (0.3\%)  \\ \hline
			\multirow{4}{*}{charging infrastructure} & \multirow{4}{*}{305 (22.3\%)}                      & charging infrastructure existence               & 191 (14.0\%) \\ \cline{3-4} 
			&                                              & charging infrastructure availability (technical) & 45 (3.3\%)  \\ \cline{3-4} 
			&                                              & charging infrastructure(general)                & 43 (3.1\%)  \\ \cline{3-4} 
			&                                              & charging infrastructure availability (physical)  & 26 (1.9\%)  \\ \hline
			range                                    & 135 (9.9\%)                                        & range                                           & 135 (9.9\%)  \\ \hline
			\multirow{4}{*}{charging technology}     & \multirow{4}{*}{119 (8.7\%)}                       & charging interfaces and technologies            & 55 (4.0\%)  \\ \cline{3-4} 
			&                                              & charging speed                                  & 30 (2.2\%)  \\ \cline{3-4} 
			&                                              & battery (other)                                 & 29 (2.1\%)  \\ \cline{3-4} 
			&                                              & range extender                                  & 5 (0.4\%)  \\ \hline
			\multirow{3}{*}{environment \& health}   & \multirow{3}{*}{71 (5.2\%)}                       & environmentally friendly car usage              & 39 (2.8\%)  \\ \cline{3-4} 
			&                                              & environment \& health (other)                   & 29 (2.1\%) \\ \cline{3-4} 
			&                                              & environmentally friendly car production         & 3 (0.2\%)  \\ \hline
			\multirow{2}{*}{society}                 & \multirow{2}{*}{283 (20.7\%)}                      & politics                                        & 171 (12.5\%) \\ \cline{3-4} 
			&                                              & desire for e-mobility                           & 112 (8.2\%)  \\ \hline
			\multirow{3}{*}{other}                   & \multirow{3}{*}{109 (8.0\%)}                       & other (miscellaneous)                           & 60 (4.4\%)  \\ \cline{3-4} 
			&                                              & definable                                       & 39 (2.8\%)  \\ \cline{3-4} 
			&                                              & joke                                            & 10 (0.7\%)  \\ 
			\hline
		\end{tabular}
	\end{adjustbox}
\end{table}
